# Supplementary material for: Closure Conversion, Flat Environments, and the Complexity of Abstract Machines
Source: arXiv:2507.15843 source file (2025-07-21)
Supplement: Supplementary file 1 [file toappendix.tex]

\gettoappendix {l:source-harmony}
\gettoappendix {l:intermediate-harmony}
\gettoappendix {l:lali-properties}
\gettoappendix {prop:intcal-key-sub-prop-rev-trans}
\gettoappendix {thm:rev-transl-implem-bricks}
\gettoappendix {cor:step-preservation}
\gettoappendix {thm:abs-impl}
\gettoappendix {l:TAM-closure-invariant}
\gettoappendix {l:TAM-decoding-invariants}
\gettoappendix {thm:sou-tam-implementation}
\gettoappendix {l:LTAM-invariants}
\gettoappendix {l:LTAM-decoding-invariants}
\gettoappendix {thm:int-ltam-implementation}
\gettoappendix {thm:tar-ttam-implementation}
\gettoappendix {prop:size-explosion-plotkin}
\gettoappendix {prop:size-explosion-tuples}
\gettoappendix {l:TAM-sub-term-invariant}
\gettoappendix {l:TAM-blue-bound}
\gettoappendix {l:TAM-overhead}
\gettoappendix {prop:TAM-number-of-trans}
\gettoappendix {thm:TAM-ram-implem}
\gettoappendix {l:LTAM-sub-term-invariant}
\gettoappendix {prop:LTAM-number-of-trans}
\gettoappendix {l:lifting-growth-bound}
